# Supplementary material for: Task Programming: Learning Data Efficient Behavior Representations
Source: arXiv:2011.13917 source file (2021-03-29)
Supplement: Supplementary file 1 [file fig_supp_efficiency.tex]

%auto-ignore

\begin{figure*}

\centering
\includegraphics[width=.33\textwidth]{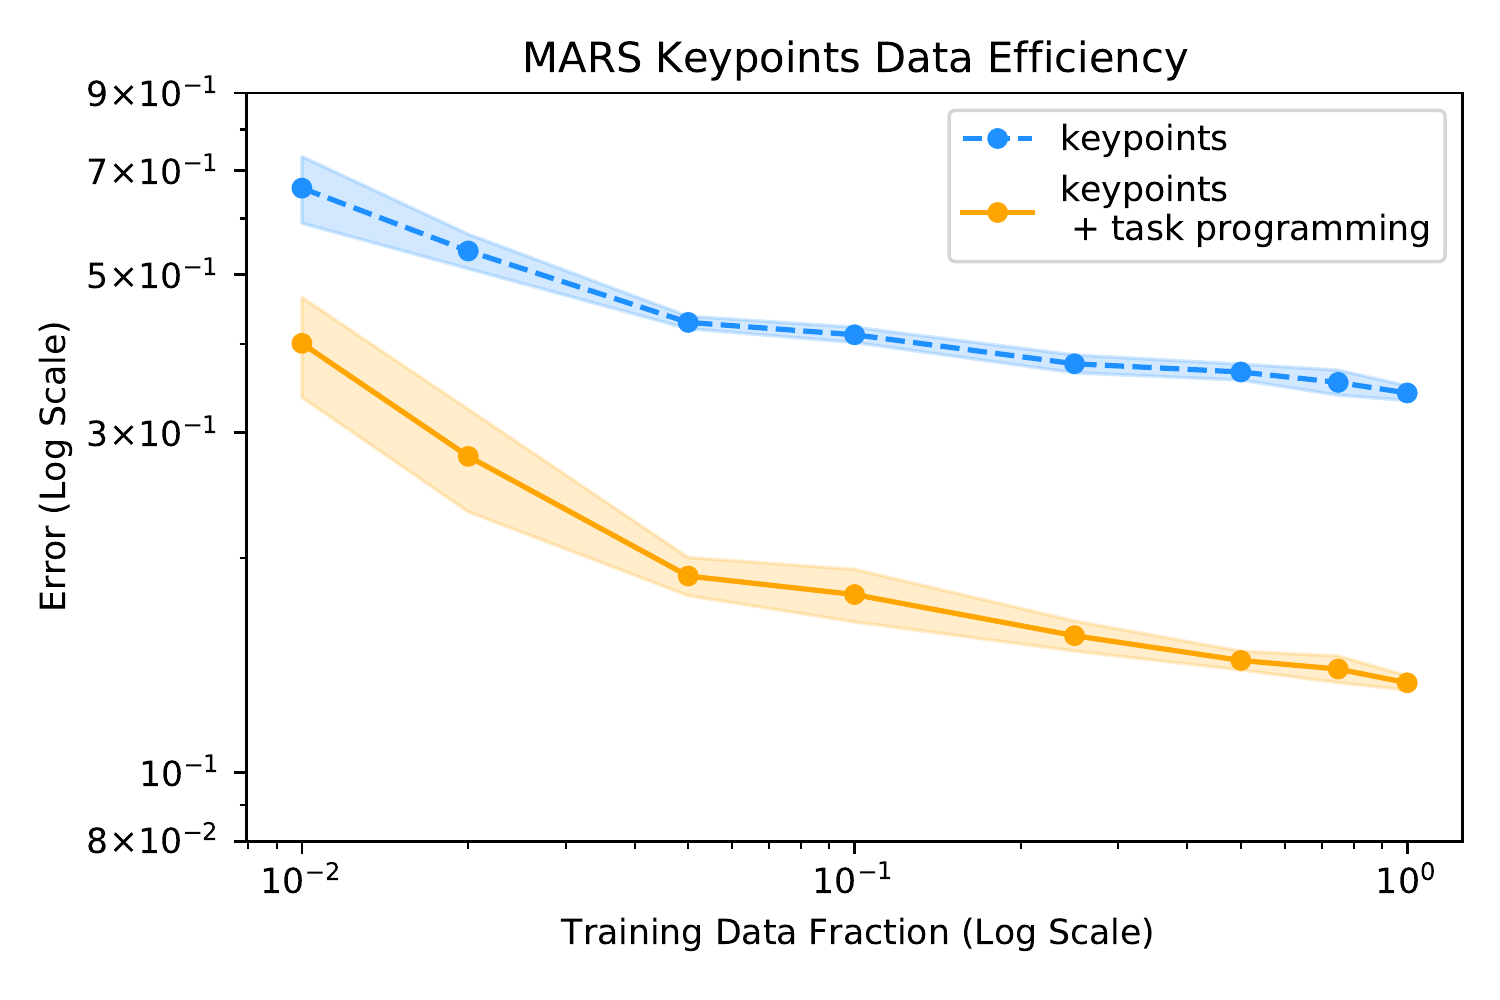}\hfill
\includegraphics[width=.33\textwidth]{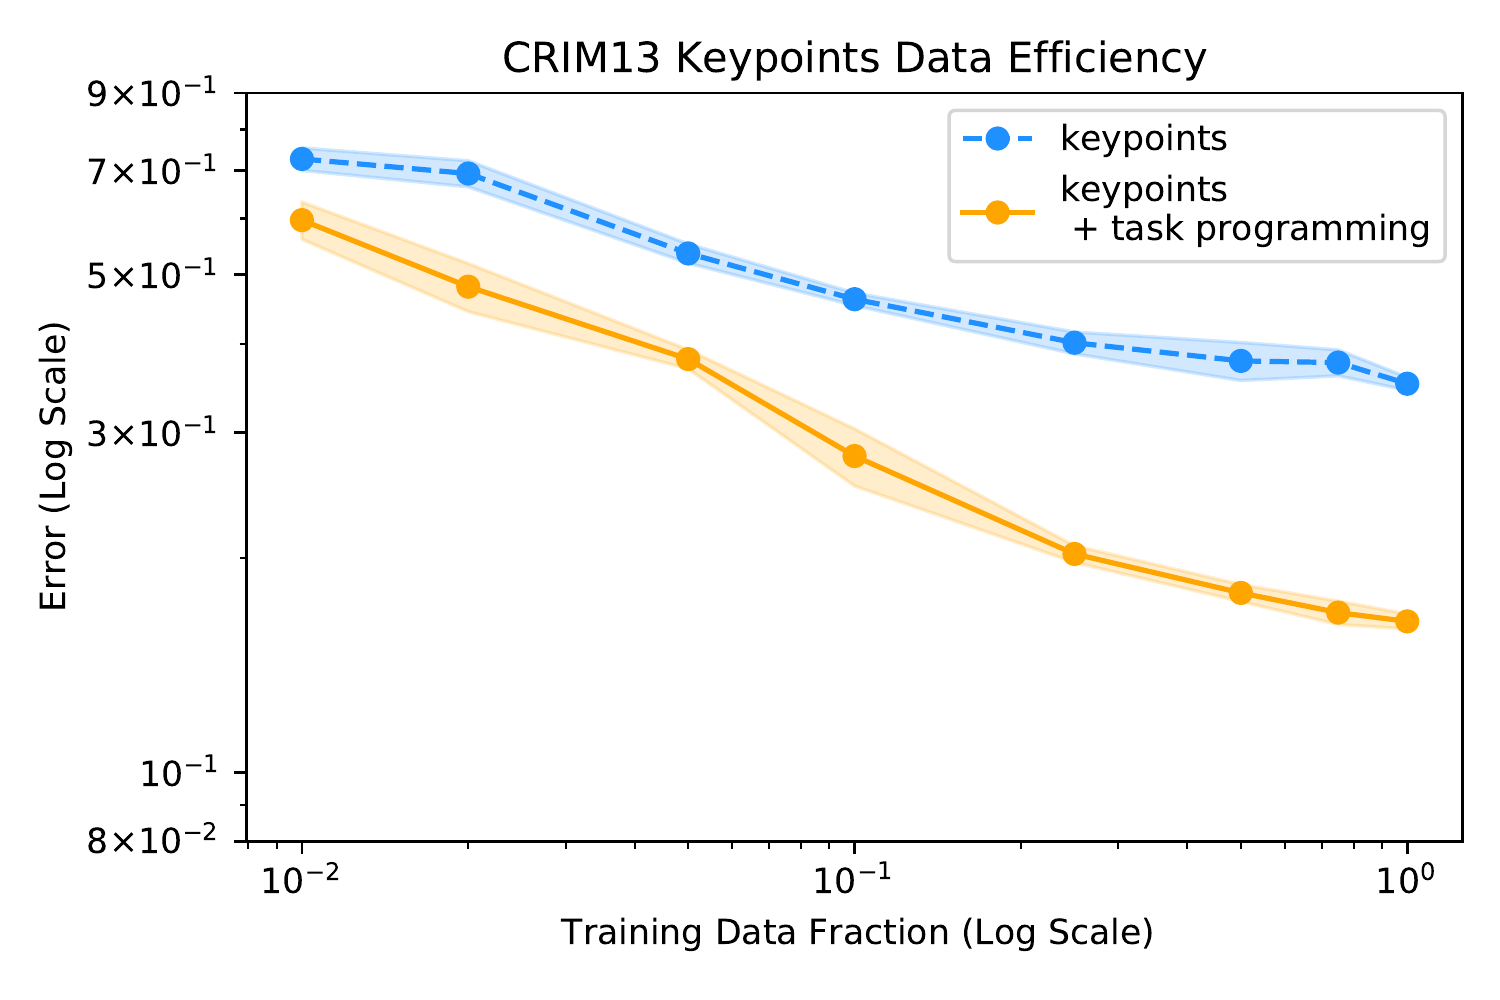}\hfill
\includegraphics[width=.33\textwidth]{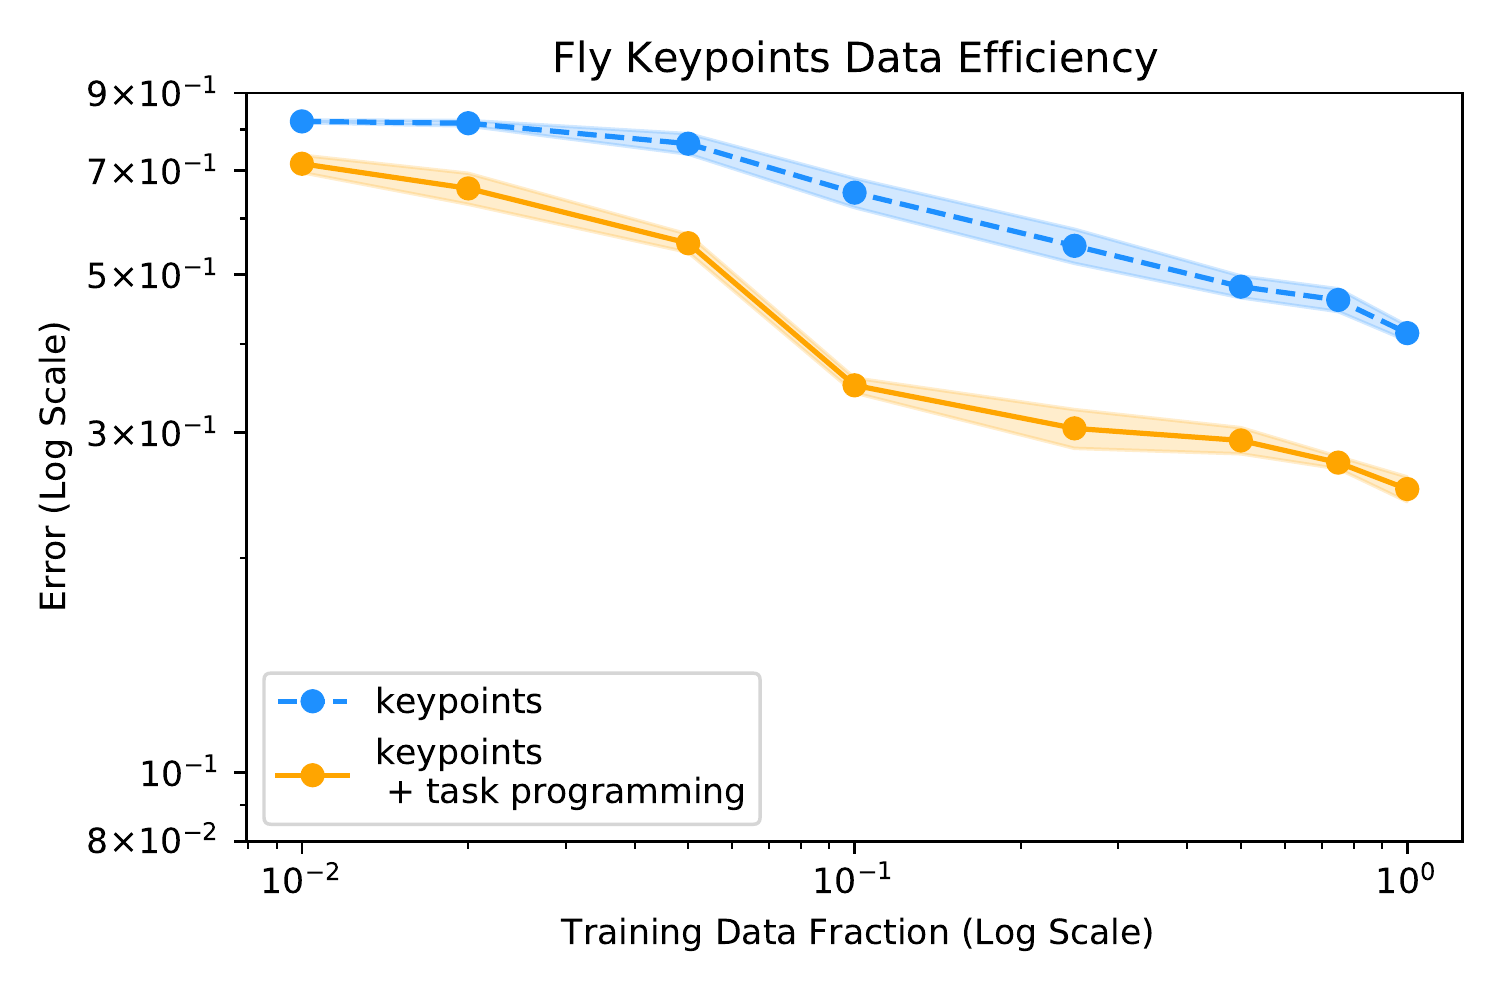}

\includegraphics[width=.33\textwidth]{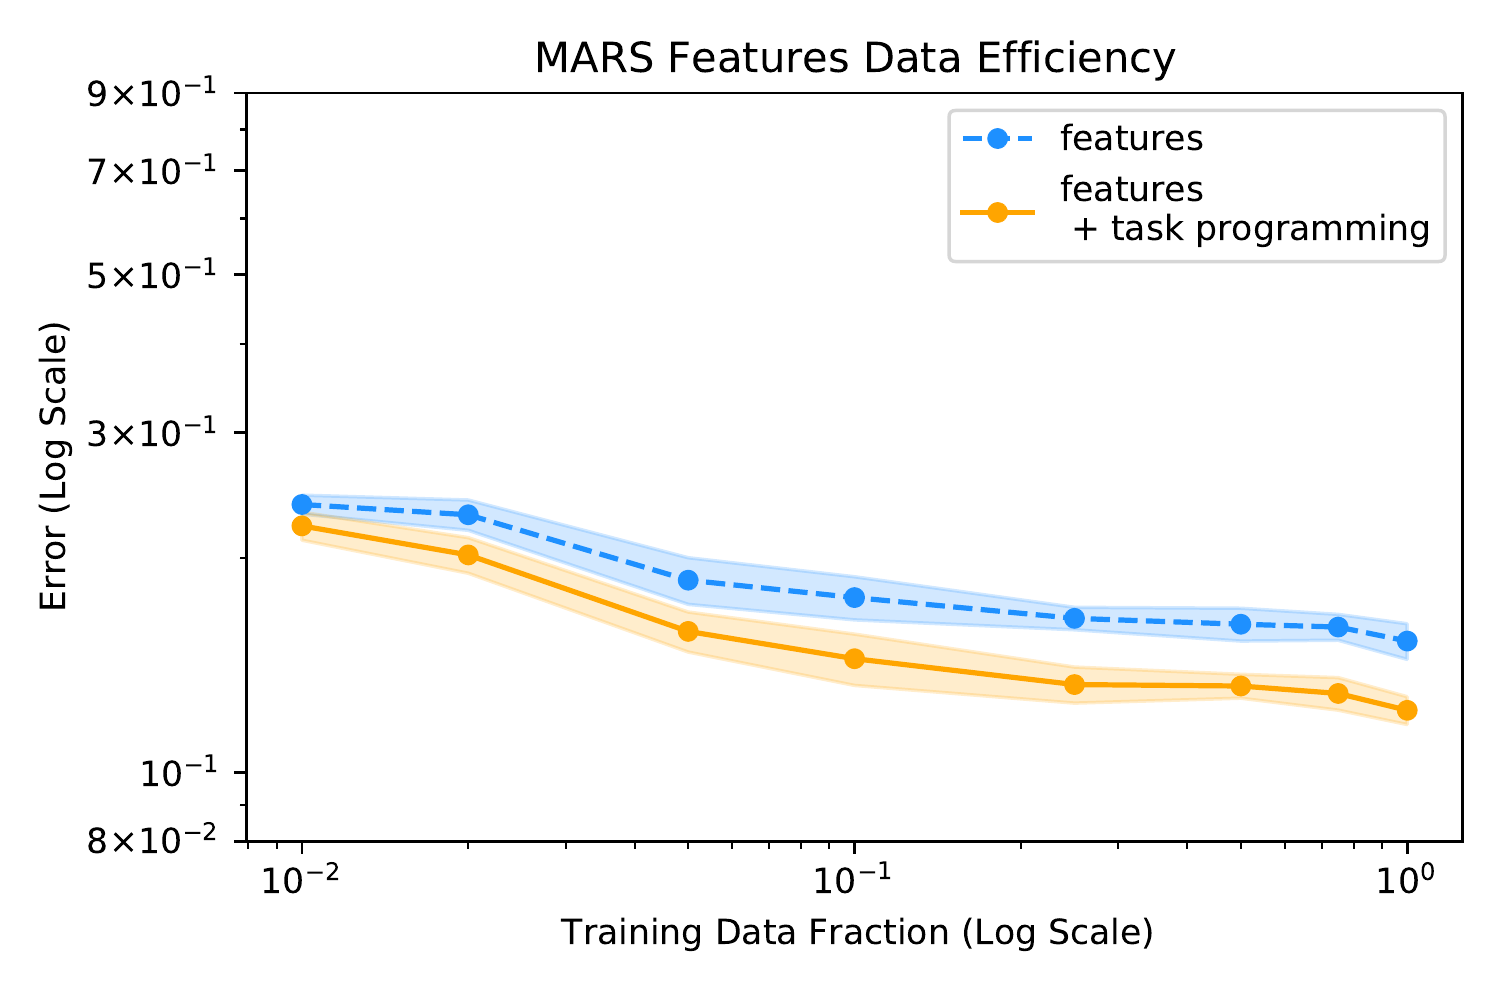}\hfill
\includegraphics[width=.33\textwidth]{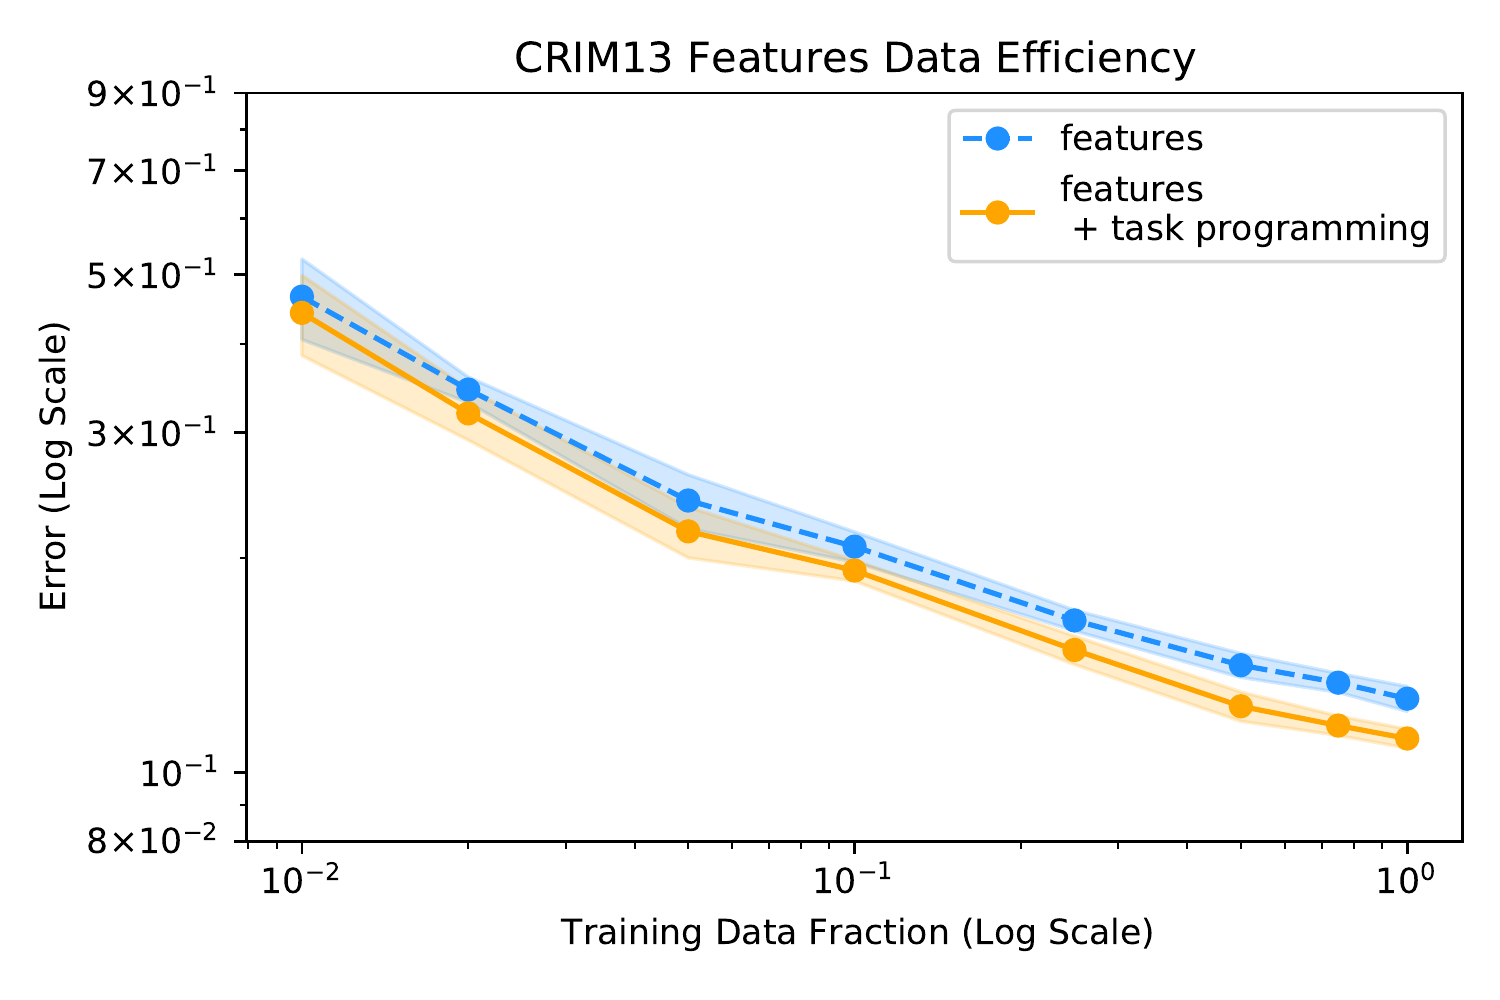}\hfill
\includegraphics[width=.33\textwidth]{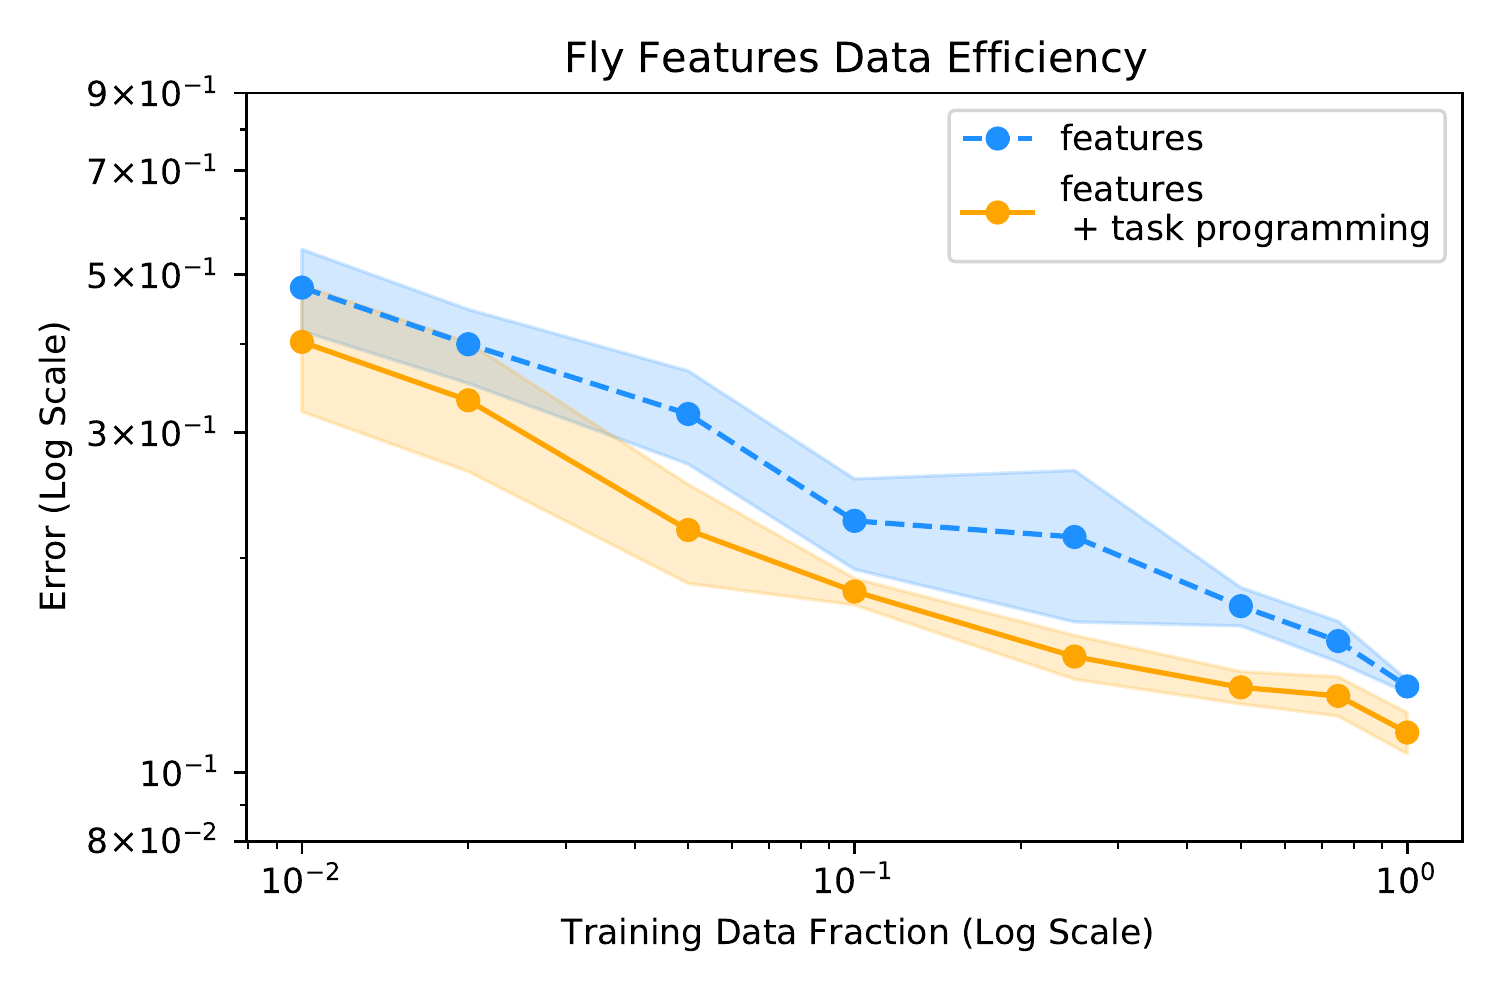}

\caption{ {\color{red} TODO: y axis ticks.} Training data fraction vs. classifier error on MARS (left), CRIM13 (middle) and fly (right). The blue dotted line represents performance with different hand-designed features, and the solid orange line represents performance with our representation. The error bars corresponds to the classifier standard deviation over 9 repeats.}
\label{fig:efficiency}

\end{figure*}

\begin{figure*}

\centering
\includegraphics[width=\textwidth]{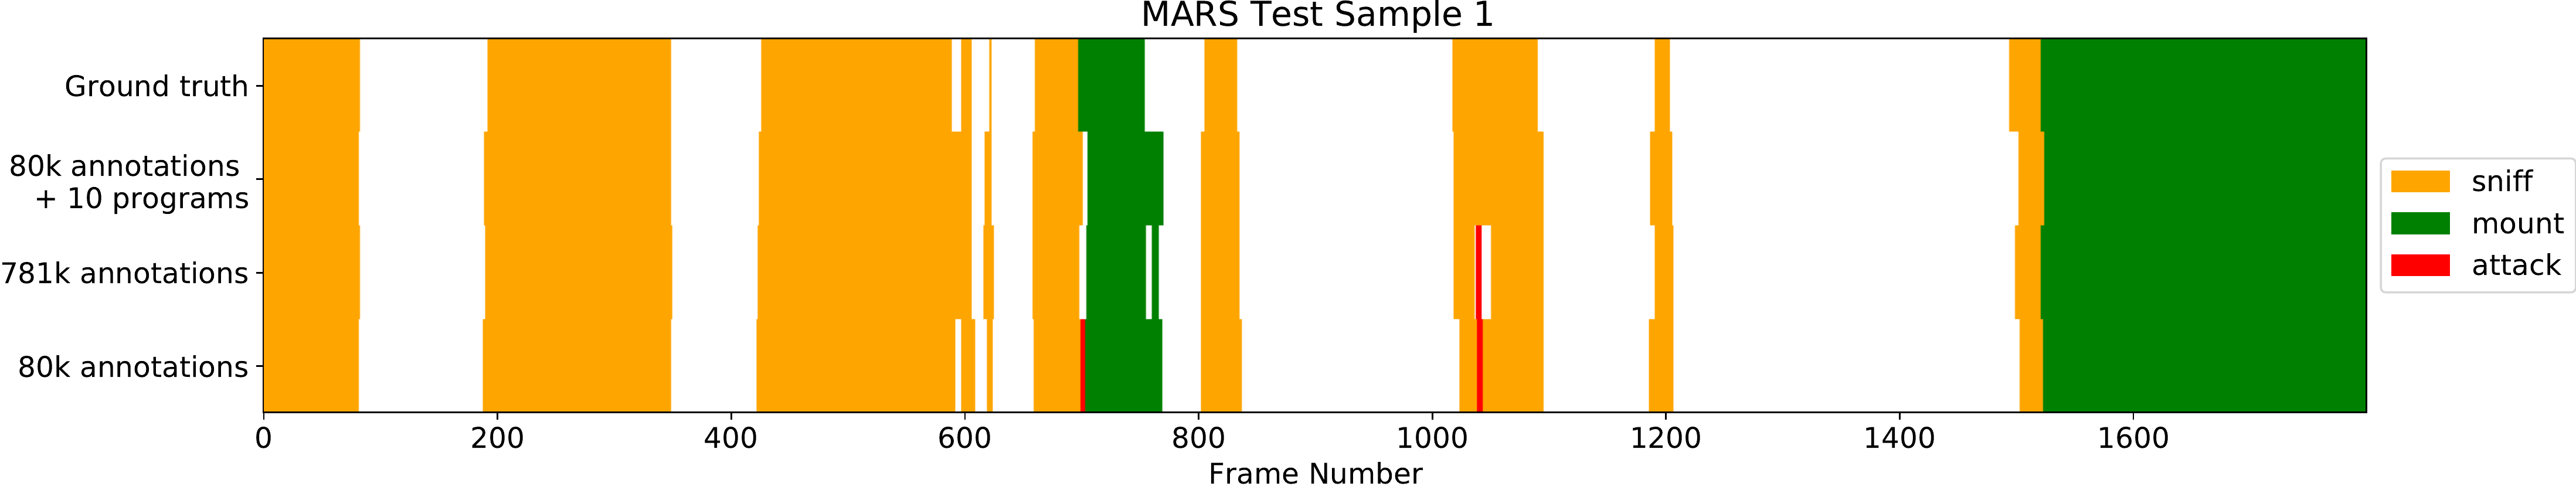}

\includegraphics[width=\textwidth]{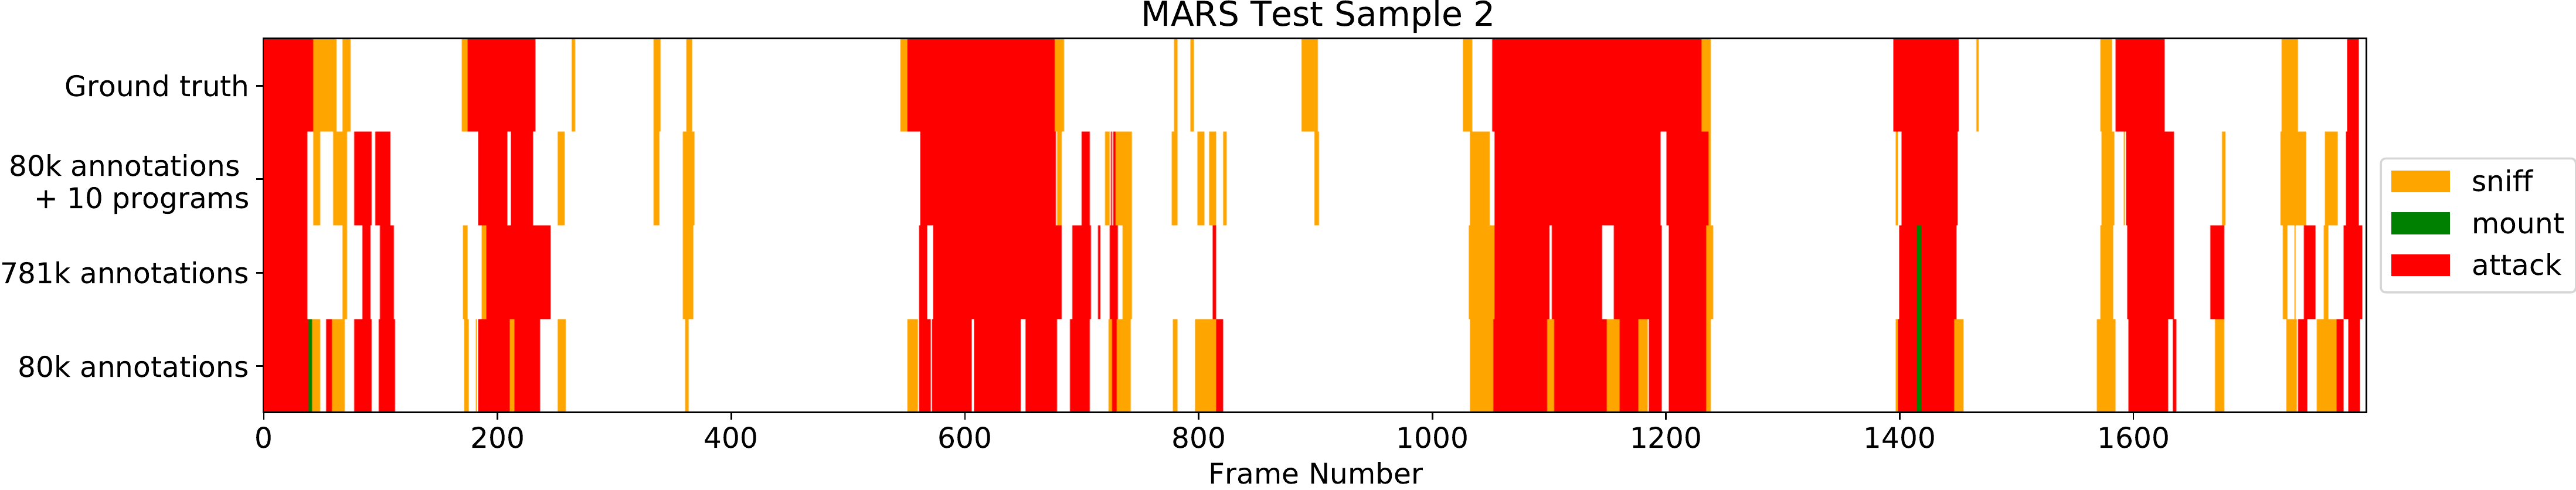}

\caption{ {\color{red} TODO: Other datasets if there is space?.} Classifier annotations on MARS dataset vs. ground truth.}
\label{fig:efficiency}

\end{figure*}
